# Supplementary material for: Quantum plasmons with optical-range frequencies in doped few-layer graphene
Source: arXiv:1703.01558 ancillary file (2018-05-03)
Supplement: Supplementary file 1 [file supplementary.pdf]

# Supplemental material

# Visible quantum plasmons in highly-doped few-layer graphene

Sharmila N. Shirodkar,[1,*] Marios Mattheakis,[1,†] Paul Cazeaux,[2]
Prineha Narang,[1,‡] Marin Soljačić,[3] and Efthimios Kaxiras[1]

[1]*John A. Paulson School of Engineering and Applied Sciences, Harvard University, Cambridge, Massachusetts 02138, USA*

[2]*School of Mathematics, University of Minnesota, Minneapolis, Minnesota 55455, USA*

[3]*Department of Physics, Massachusetts Institute of Technology, 77 Massachusetts Avenue, Cambridge, Massachusetts 02139, USA*

(Dated: November 3, 2017)

## TRANSPARENT BOUNDARY CONDITIONS

The potential $\phi(\mathbf{r},\omega)$ and charge density $\rho(\mathbf{r},\omega)$ of quantum plasmon modes are obtained as left and right eigenfunctions (which satisfy the Poisson equation) of the dielectric operator $\hat{\epsilon}(\omega)$, diagonalized in the plane wave basis:

$$\hat{\epsilon}(\omega)\phi_n(\omega) = [\hat{1} - \hat{v}\ \hat{\chi}^0(\omega)]\phi_n(\omega) = \lambda_n(\omega)\phi_n(\omega) \tag{1}$$

with the dielectric operator $\hat{\epsilon}(\omega)$ expressed in terms of the non-interacting linear response operator $\hat{\chi}^0(\omega)$ and the Coulomb interaction operator $\hat{v} = 1/|\mathbf{r} - \mathbf{r}'|$. The condition for observing a plasmon at frequency $\omega_\mathrm{p}$ is that the real part of the dielectric function, $\mathrm{Re}[\lambda_n(\omega)]$, goes to 0 from a negative value. Hence, $\mathrm{Re}[\lambda_n(\omega = \omega_\mathrm{p})] = 0$ is the condition for observing a plasmon.

Rearranging eq. 1 in terms of $\hat{\chi}^0(\omega)$ we get,

$$\hat{\chi}^0(\omega)\phi_n(\omega) = \frac{1-\lambda_n}{4\pi}\hat{v}^{-1}\phi_n(\omega) \tag{2}$$

The reciprocal space representation of the linear response operator [under the random phase approximation (RPA)] is a matrix $\chi^0_{\mathbf{G},\mathbf{G}'}(\mathbf{q},\omega)$, where $\mathbf{G}$ and $\mathbf{G}'$ are vectors belonging to the reciprocal lattice, $\mathbf{q}$ is the plasmonic in-plane ($xy$) wave vector, and $\omega$ is the frequency. The reciprocal space representation of the Coulomb interaction operator is given by:

$$\hat{v}_{\mathbf{G},\mathbf{G}'}(\mathbf{q}) = \frac{4\pi}{|\mathbf{q}+\mathbf{G}|^2}\delta_{\mathbf{G},\mathbf{G}'}, \text{inverting we get,} \tag{3}$$

$$\hat{v}^{-1}_{\mathbf{G},\mathbf{G}'}(\mathbf{q}) = \frac{|\mathbf{q}+\mathbf{G}|^2}{4\pi}\delta_{\mathbf{G},\mathbf{G}'}, \tag{4}$$

In ideal 2D materials, the vacuum $\rightarrow \infty$ implying $\phi(\mathbf{r},\omega)$ and $\rho(\mathbf{r},\omega)$ exponentially decay with distance perpendicular to the plane of the material. In *ab-initio* calculations, the vacuum is simulated by placing the 2D material in a rectangular cell with large spacing (typically $\geq$ 10 Å) or more along the direction perpendicular to the sheet (*i.e.* $z$ axis). Let $z_-$, $z_+$ be the bounds of the super-cell (simulation box) along the $z$ direction, where the 2D material is placed at the center of the box at $z = (z_+ - z_-)/2$. Since, the bounds of the simulation cell are along the $z$ direction, we take one dimensional fourier transform along this direction to get a real space representation in this coordinate. The one dimensional

fourier transform of $\hat{v}^{-1}_{\mathbf{G},\mathbf{G}'}(\mathbf{q})$ is given as follows,

$$\begin{aligned}
\hat{v}^{-1}_{\mathbf{G}_{\rm xy},\mathbf{G}'_{\rm xy}}(\mathbf{q},z,z') &= \frac{1}{4\pi}\sum_{\mathbf{G}_{\rm z},\mathbf{G}'_{\rm z}}\left(|\mathbf{q}+\mathbf{G}_{\rm xy}|^2+|\mathbf{G}_{\rm z}|^2\right)e^{i(zG_z-z'G'_z)}\delta_{\mathbf{G}_{\rm xy},\mathbf{G}'_{\rm xy}}\delta_{\mathbf{G}_{\rm z},\mathbf{G}'_{\rm z}},\\
&= \frac{1}{4\pi}\sum_{\mathbf{G}_{\rm z}}\left(|\mathbf{q}+\mathbf{G}_{\rm xy}|^2+|\mathbf{G}_{\rm z}|^2\right)e^{iG_z(z-z')}\delta_{\mathbf{G}_{\rm xy},\mathbf{G}'_{\rm xy}},\\
&= \frac{1}{4\pi}\left[\left(|\mathbf{q}+\mathbf{G}_{\rm xy}|^2\right)\sum_{\mathbf{G}_{\rm z}}e^{iG_z(z-z')}+\sum_{\mathbf{G}_{\rm z}}|\mathbf{G}_{\rm z}|^2e^{iG_z(z-z')}\right]\delta_{\mathbf{G}_{\rm xy},\mathbf{G}'_{\rm xy}},\\
&= \frac{1}{4\pi}\left[\left(|\mathbf{q}+\mathbf{G}_{\rm xy}|^2\right)\sum_{\mathbf{G}_{\rm z}}e^{iG_z(z-z')}+\sum_{\mathbf{G}_{\rm z}}\left(-\frac{\partial^2}{\partial z^2}\right)e^{iG_z(z-z')}\right]\delta_{\mathbf{G}_{\rm xy},\mathbf{G}'_{\rm xy}},\\
&= \frac{1}{4\pi}\left(|\mathbf{q}+\mathbf{G}_{\rm xy}|^2-\frac{\partial^2}{\partial z^2}\right)\delta_{\mathbf{G}_{\rm xy},\mathbf{G}'_{\rm xy}}\sum_{\mathbf{G}_{\rm z}}e^{iG_z(z-z')},\\
&= \frac{1}{4\pi}\left(|\mathbf{q}+\mathbf{G}_{\rm xy}|^2-\frac{\partial^2}{\partial z^2}\right)\delta_{\mathbf{G}_{\rm xy},\mathbf{G}'_{\rm xy}}\delta(z-z').
\end{aligned} \tag{5}$$

Substituting eq. 5 in eq. 2 we get:

$$\hat{\chi}^0\phi_n(z,\mathbf{G}_{\rm xy},\mathbf{q},\omega) = \frac{1-\lambda_n}{4\pi}\left(|\mathbf{q}+\mathbf{G}_{\rm xy}|^2-\frac{\partial^2}{\partial z^2}\right)\phi_n(z,\mathbf{G}_{\rm xy},\mathbf{q},\omega), \tag{6}$$

The left-hand side vanishes in the vacuum region (no response, *i.e.* $\chi^0$ is 0 for $z > z_+$, $z < z_-$), and equation (6) reduces to the one-dimensional Poisson equation. For any nonzero value of $|\mathbf{q}+\mathbf{G}_{\rm xy}|$, we thus obtain an explicit solution

$$\begin{aligned}
\phi_n(z,\mathbf{G}_{\rm xy},\mathbf{q},\omega) &= \phi_n(z_-,\mathbf{G}_{\rm xy},\mathbf{q},\omega)e^{-|\mathbf{q}+\mathbf{G}_{\rm xy}|(z_--z)} \qquad \text{for } z\le z_-,\\
\phi_n(z,\mathbf{G}_{\rm xy},\mathbf{q},\omega) &= \phi_n(z_+,\mathbf{G}_{\rm xy},\mathbf{q},\omega)e^{-|\mathbf{q}+\mathbf{G}_{\rm xy}|(z-z_+)} \qquad \text{for } z\ge z_+.
\end{aligned} \tag{7}$$

The $\hat{\chi}^0$ in eqs. 6 and 7 is the one dimensional fourier transform as follows,

$$\hat{\chi}^0\phi(z,\mathbf{G}_{\rm xy},\mathbf{q},\omega) = \int_{z_-}^{z_+}\sum_{\mathbf{G}'_{\rm xy}}\chi^0_{\mathbf{G}_{\rm xy},\mathbf{G}'_{\rm xy}}(z,z',\mathbf{q},\omega)\phi(z',\mathbf{G}'_{\rm xy},\mathbf{q},\omega)\mathrm{d}z'. \tag{8}$$

Solving eigenvalue eq. 6 using $\chi^0$ computed using first-principles DFT simulations, we obtain $\lambda_n$ and $\phi_n$ as eigenvalues and eigenvectors. However, the long-range nature of Coulomb term gives rise to interaction between the periodic images of the plasmons (along $z$ direction) even with the implementation of exact coulomb cutoff [1]. This is seen through the non-decaying $\phi(\mathbf{r},\omega)$, and finite and spurious $\rho(\mathbf{r},\omega)$ at the vacuum edges [see Fig. 2 (a) and Fig. 2(d) in main manuscript], implying that $\phi(\mathbf{r},\omega) \not\to 0$ as $z\to\pm\infty$. However, by implementing additional constraints on the potential function $\phi_n$ we overcome this issue, and we term the additional constraints as 'transparent boundary conditions'.

The transparent boundary conditions impose the continuity of $\phi_n$ and its first derivative with respect to $z$ at $z = z_\pm$ (in eq. 7). Thus giving,

$$\frac{\partial \phi_n}{\partial z}(\mathbf{q}, \mathbf{G}_{\text{xy}}, z_\pm, \omega) = \mp|\mathbf{q} + \mathbf{G}_{\text{xy}}|\phi_n(\mathbf{q}, \mathbf{G}_{\text{xy}}, z_\pm, \omega), \tag{9}$$

which implies that the charge density and potential do not see the periodic boundary along $z$ direction for any value of $\mathbf{q}$, and hence decay to zero as $z \to \pm\infty$. This simplifies to solving eq. 6 with modified $\hat{v}^{-1}_{\mathbf{G}_{\text{xy}},\mathbf{G}'_{\text{xy}}}(\mathbf{q}, z, z')$ implemented using finite differences, given by the matrix below.

$$\hat{v}^{-1}_{\mathbf{G}_{\text{xy}},\mathbf{G}'_{\text{xy}}}(\mathbf{q}, z) = \begin{bmatrix} \frac{g^2}{2} + \frac{1}{dz^2} + \frac{g}{dz}, & \frac{-1}{dz^2}, & 0, & 0, & 0, & \dots \\ \frac{-1}{dz^2}, & g^2 + \frac{2}{dz^2}, & \frac{-1}{dz^2}, & 0, & 0, & \dots \\ 0, & \frac{-1}{dz^2}, & g^2 + \frac{2}{dz^2}, & \frac{-1}{dz^2}, & 0, & \dots \\ \vdots & \vdots & \vdots & \vdots & \vdots & \vdots \\ \dots & 0, & \frac{-1}{dz^2}, & g^2 + \frac{2}{dz^2}, & \frac{-1}{dz^2}, & 0 \\ \dots & 0, & 0, & \frac{-1}{dz^2}, & g^2 + \frac{2}{dz^2}, & \frac{-1}{dz^2} \\ \dots & 0, & 0, & 0, & \frac{-1}{dz^2}, & \frac{g^2}{2} + \frac{1}{dz^2} + \frac{g}{dz} \end{bmatrix} \delta_{\mathbf{G}_{\text{xy}},\mathbf{G}'_{\text{xy}}}$$

## DETAILS OF $\tau$ CALCULATIONS

The intrinsic carrier relaxation rate in materials is determined by two prominent processes, electron-phonon (e-ph) scattering and electron-electron (e-e) scattering. Here we formally describe the theoretical and computational methodology used in the paper.

**Electron-electron scattering:** For the electron-electron scattering contribution, we calculate the imaginary part of the quasiparticle self energy given by [2],

$$\text{Im}\,\Sigma^{\text{e-e}}_{\mathbf{q}n} = \int_{\text{BZ}} \frac{d\mathbf{q}'}{(2\pi)^3} \sum_{n'} \sum_{\mathbf{G}\mathbf{G}'} \tilde{\rho}_{\mathbf{q}'n',\mathbf{q}n}(\mathbf{G}) \tilde{\rho}^*_{\mathbf{q}'n',\mathbf{q}n}(\mathbf{G}') \times \frac{4\pi e^2}{|\mathbf{q}' - \mathbf{q} + \mathbf{G}|^2} \text{Im}\left[\epsilon^{-1}_{\mathbf{G}\mathbf{G}'}(\mathbf{q}' - \mathbf{q}, \varepsilon_{\mathbf{q}n} - \varepsilon_{\mathbf{q}'n'})\right], \tag{10}$$

where $\tilde{\rho}_{\mathbf{q}'n',\mathbf{q}n}(\mathbf{G})$ is the plane-wave expansion of the product density $\sum_\sigma u^{\sigma *}_{\mathbf{q}'n'}(\mathbf{r}) u^\sigma_{\mathbf{q}n}(\mathbf{r})$ of Bloch functions with reciprocal lattice vectors $\mathbf{G}$, and $\epsilon^{-1}_{\mathbf{G}\mathbf{G}'}(\mathbf{k}, \omega)$ is the microscopic dielectric function in a plane-wave basis calculated within the random-phase approximation. See Ref. [2] for a detailed exposition. The connection to Fermi's golden rule for electron-electron

scattering is discussed next. Here, we calculate (10) in JDFTx[3] using an explicit frequency integral for the dielectric function, retaining local field effects.

**Electron-phonon scattering:** We calculate the electron-phonon scattering contribution to the electron linewidth using the Fermi golden rule

$$\mathrm{Im}\,\Sigma^{\text{e-ph}}_{\mathbf{q}n} = \pi \int_{\mathsf{BZ}} \frac{\Omega d\mathbf{q}'}{(2\pi)^3} \sum_{n'\alpha\pm} \left( n_{\mathbf{q}'-\mathbf{q},\alpha} + \frac{1}{2} \mp \frac{1}{2} \right) \times \delta(\varepsilon_{\mathbf{q}'n'} - \varepsilon_{\mathbf{q}n} \mp \hbar\omega_{\mathbf{q}'-\mathbf{q},\alpha}) \left| g^{\mathbf{q}'-\mathbf{q},\alpha}_{\mathbf{q}'n',\mathbf{q}n} \right|^2, \quad (11)$$

**Scattering to Rate Calculations:** Stated a different way, the Fermi's Golden rule for electron-phonon scattering yields the rate:

$$\left(\tau^{-1}_{\text{e-ph}}\right)_{\mathbf{q}n} = \frac{2\pi}{\hbar} \int_{\mathsf{BZ}} \frac{\Omega d\mathbf{q}'}{(2\pi)^3} \sum_{n'\alpha\pm} \delta(E_{\mathbf{q}'n'} - E_{\mathbf{q}n} \mp \hbar\omega_{\mathbf{q}'-\mathbf{q},\alpha}) \times \left( n_{\mathbf{q}'-\mathbf{q},\alpha} + \frac{1}{2} \mp \left( \frac{1}{2} - f_{\mathbf{q}'n'} \right) \right) \left| g^{\mathbf{q}'-\mathbf{q},\alpha}_{\mathbf{q}'n',\mathbf{q}n} \right|^2. \quad (12)$$

Above, electronic states with energies $E_{\mathbf{q}'n'}$ and Fermi-Dirac occupation factors $f_{\mathbf{q}n}$ are labeled by wave-vectors $\mathbf{q}, \mathbf{q}'$ in the Brillouin zone (BZ) and band indices $n, n'$. Phonon states with energies $\hbar\omega_{\mathbf{k}\alpha}$ and Bose-Einstein occupation factors $n_{\mathbf{k}\alpha}$ are labelled by wave-vectors $\mathbf{k}$ ($= \mathbf{q}' - \mathbf{q}$ by momentum conservation) and polarization index $\alpha$. The electron-phonon matrix elements $g^{\mathbf{q}'-\mathbf{q},\alpha}_{\mathbf{q}'n',\mathbf{q}n}$ couple two electronic states with a phonon mode as in the 3-vertex in the Feynman diagram representation.

On the other hand, the rate for electron-electron scattering is given by[2, 4]

$$\left(\tau^{-1}_{\text{e-e}}\right)_{\mathbf{q}n} = \frac{2\pi}{\hbar} \int_{\mathsf{BZ}} \frac{d\mathbf{q}'}{(2\pi)^3} \sum_{n'} \sum_{\mathbf{G}\mathbf{G}'} \tilde{\rho}_{\mathbf{q}'n',\mathbf{q}n}(\mathbf{G}) \tilde{\rho}^*_{\mathbf{q}'n',\mathbf{q}n}(\mathbf{G}') \times \frac{1}{\pi} \mathrm{Im} \Bigg[ \underbrace{\frac{4\pi e^2}{|\mathbf{q}' - \mathbf{q} + \mathbf{G}|^2} \epsilon^{-1}_{\mathbf{G}\mathbf{G}'}(\mathbf{q}' - \mathbf{q}, E_{\mathbf{q}n} - E_{\mathbf{q}'n'})}_{W_{\mathbf{G}\mathbf{G}'}(\mathbf{q}'-\mathbf{q}, E_{\mathbf{q}n} - E_{\mathbf{q}'n'})} \Bigg]. \quad (13)$$

Above, the relevant matrix element for Fermi's golden rule is obtained by the overlap of the density matrix $\tilde{\rho}_{\mathbf{q}'n',\mathbf{q}n}$ between initial and final electronic wavefunctions, expanded in the plane-wave basis with reciprocal lattice vectors $\mathbf{G}$, with the imaginary part of the dynamically screened Coulomb operator $W_{\mathbf{G}\mathbf{G}'}(\mathbf{q}' - \mathbf{q}, \hbar\omega)$. This operator is written in terms of the electronic dielectric function, which in turn, is derived from the electronic density matrices and energies. Note that the density matrices contain the lower incoming and outgoing electronic states while $\mathrm{Im}\, W$ contains the virtual photon propagator and the upper electronic states. See Ref. [2] for a detailed exposition and Ref. [4, 5] for implementation details.

Further computational details: We perform *ab initio* density-functional theory (DFT) calculations of the electronic band structure, phonon dispersion relations and electron-phonon matrix elements used in (12-13). We use maximally-localized Wannier functions[6] to interpolate all the DFT-calculated quantities from a coarser Brillouin zone mesh ($24 \times 24 \times 4$) to the much finer meshes ($600 \times 600 \times 12$), which is critical for accurately resolving the phonon energy scales in *ab initio* calculations of electron-phonon properties.

## PLOTS

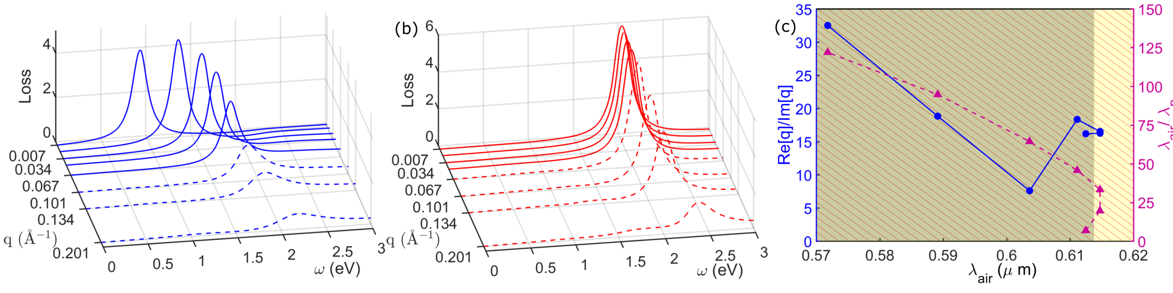


FIG. S1. Loss function for, (a) symmetric mode (blue) and (b) antisymmetric mode (red) for G/Li/G system. Solid and dashed lines denote modes undamped and overdamped by interband transitions. (c) Re[$q$]/Im[$q$] (left axis, circles with solid line in blue), and field localization (right axis, triangles with dashed line in magenta) or wave "shrinkage"of the antisymmetric mode. The grey shaded areas denote the region of inter-band losses, and the yellow shaded (hatched) areas denote the visible frequency range, calculated with the Fermi velocity of graphene. $\tau$ is $\approx$ 29 fs.

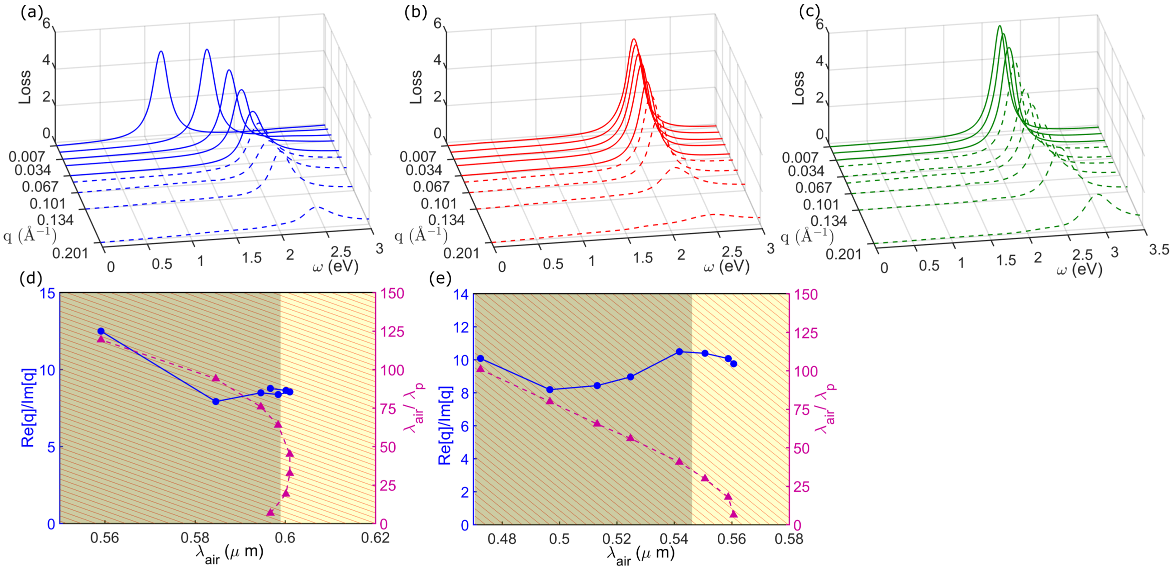


FIG. S2. Loss function for, (a) symmetric mode (blue), (b) antisymmetric mode (red) and (c) second symmteric mode (green) for G/Li/G/Li/G system. Solid and dashed lines denote modes undamped and overdamped by interband transitions. $\mathrm{Re}[q]/\mathrm{Im}[q]$ (left axis, circles with solid line in blue), and field localization (right axis, triangles with dashed line in magenta) or wave “shrinkage”) of the (d) antisymmetric mode and (e) second symmetric mode. The grey shaded areas denote the region of inter-band losses, and the yellow shaded (hatched) areas denote the visible frequency range, calculated with the Fermi velocity of graphene. $\tau$ is $\approx$ 19 fs.

* Present address: Department of Materials Science and NanoEngineering, Rice University, Houston, TX 77005, USA; sns8@rice.edu

† Department of Physics, University of Crete, PO, Box 2208, 71003 Heraklion, Greece

‡ Faculty of Arts and Sciences, Harvard University, Cambridge MA 02138, USA

[1] C. A. Rozzi, D. Varsano, A. Marini, E. K. U. Gross, and A. Rubio, Phys. Rev. B **73**, 205119 (2006).

[2] F. Ladstädter, U. Hohenester, P. Puschnig, and C. Ambrosch-Draxl, Phys. Rev. B **70**, 235125 (2004).

[3] R. Sundararaman, D. Gunceler, K. Letchworth-Weaver, K. A. Schwarz, and T. A. Arias, "JDFTx," `http://jdftx.sourceforge.net` (2012).

[4] A. Brown, R. Sundararaman, P. Narang, W. A. Goddard III, and H. A. Atwater, ACS Nano **10**, 957 (2016).

[5] P. Narang, L. Zhao, S. Claybrook, and R. Sundararaman, Adv. Opt. Mater. **5**, 1600914 (2017).

[6] I. Souza, N. Marzari, and D. Vanderbilt, Phys. Rev. B **65**, 035109 (2001).
